# Supplementary material for: Electron-phonon coupling and momentum-dependent electron dynamics in EuFe2As2 using time- and angle-resolved photoemission spectroscopy
Source: arXiv:1008.1561 source file (2010-12-06)
Supplement: Supplementary file 1 [file Rettig_FeAs_SOM_resubm.pdf]

# Supporting Online Material

**for**

## ***"Electron-phonon coupling and momentum-dependent electron dynamics in $EuFe_2As_2$ using time- and angle-resolved photoemission spectroscopy"***

L. Rettig, R. Cortés, S. Thirupathaiah, P. Gegenwart, H.S. Jeevan,
T. Wolf, U. Bovensiepen, M. Wolf, H.A. Dürr, and J. Fink

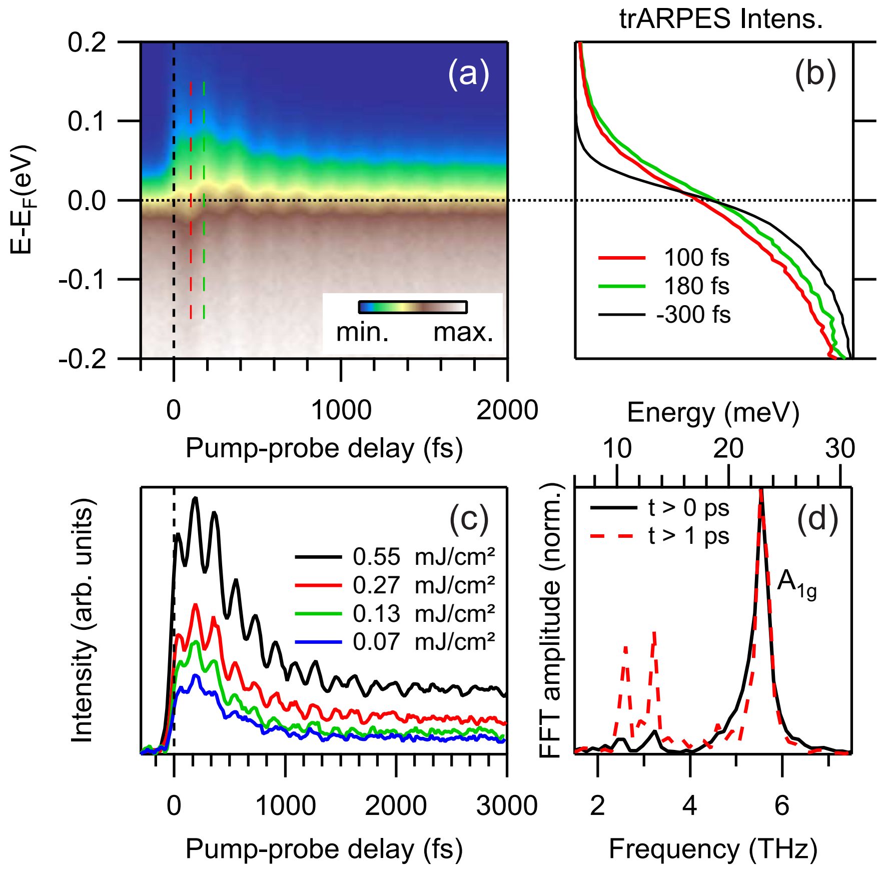


FIG. S1. (a) trARPES signal of $BaFe_{1.85}Co_{0.15}As_2$ near the Γ-point using an absorbed fluence of $F$=0.55 mJ/cm$^2$, as a function of energy and pump-probe delay. Dashed lines mark spectra shown in (b). (b) trARPES spectra from the data in (a) for a minimum (red) and maximum (green) of the $A_{1g}$ oscillation in comparison to a spectrum before excitation (black). Note the rigorous shift of the Fermi cutoff by the oscillation. (c) Integrated trARPES intensity for $E > E_F$ and various fluences. (d) Normalized fast Fourier transform of the $F$=0.55 mJ/cm$^2$ data in (c), for $t > 0$ ps (solid line), showing the same three modes observed in $EuFe_2As_2$. Taking only data with $t > 1$ ps into account (dashed line) reveals a shorter lifetime of the $A_{1g}$ mode with respect to the two lower frequency modes.

The coherent oscillations of the spectral weight near the Fermi level observed by time- and angle-resolved photoemission spectroscopy (trARPES) in $EuFe_2As_2$ [1] are also observed in other 122 Fe pnictide compounds. All three coherent modes were found in superconducting samples of $BaFe_{1.85}Co_{0.15}As_2$ ($T_c$=23.5 K) [2] and undoped $BaFe_2As_2$. trARPES data of

$BaFe_{1.85}Co_{0.15}As_2$ near the Fermi level are shown in Fig. S1(a) for comparable experimental conditions as for data of $EuFe_2As_2$ [1]. Panel (b) shows energy distribution curves for delays corresponding to a minimum (100 fs) and maximum (180 fs) of the 5.6 THz oscillation in comparison to a spectrum before excitation. Besides a pronounced change of the electronic distribution function due to excited electrons, the rigid shift of the spectra with the oscillation phase demonstrates, that the coherent modes directly modulate the transient chemical potential. Like in $EuFe_2As_2$, a longer lifetime is found for the two lower frequency modes compared to the decay of the $A_{1g}$ mode from fast Fourier transformation analysis (Fig. S1(d)).

[1] L. Rettig *et al.*, submitted (2010).

[2] F. Hardy *et al.*, Phys. Rev. Lett., **102**, 187004 (2009).
